# Supplementary material for: Geometry-Guided Street-View Panorama Synthesis from Satellite Imagery
Source: arXiv:2103.01623 source file (2022-03-26)
Supplement: Supplementary file 1 [file supple.tex]

\documentclass[10pt,journal,compsoc]{IEEEtran}
%
% If IEEEtran.cls has not been installed into the LaTeX system files,
% manually specify the path to it like:
% \documentclass[10pt,journal,compsoc]{.._sty_IEEEtran}

\usepackage{subfig}
\usepackage{graphicx}

% Some very useful LaTeX packages include:
% (uncomment the ones you want to load)

% *** MISC UTILITY PACKAGES ***
%
%\usepackage{ifpdf}
% Heiko Oberdiek's ifpdf.sty is very useful if you need conditional
% compilation based on whether the output is pdf or dvi.
% usage:
% \ifpdf
%   % pdf code
% \else
%   % dvi code
% \fi
% The latest version of ifpdf.sty can be obtained from:
% http:__www.ctan.org_pkg_ifpdf
% Also, note that IEEEtran.cls V1.7 and later provides a builtin
% \ifCLASSINFOpdf conditional that works the same way.
% When switching from latex to pdflatex and vice-versa, the compiler may
% have to be run twice to clear warning_error messages.

% *** CITATION PACKAGES ***
%
\ifCLASSOPTIONcompsoc
  % IEEE Computer Society needs nocompress option
  % requires cite.sty v4.0 or later (November 2003)
  \usepackage[nocompress]{cite}
\else
  % normal IEEE
  \usepackage{cite}
\fi
% cite.sty was written by Donald Arseneau
% V1.6 and later of IEEEtran pre-defines the format of the cite.sty package
% \cite{} output to follow that of the IEEE. Loading the cite package will
% result in citation numbers being automatically sorted and properly
% "compressed_ranged". e.g., [1], [9], [2], [7], [5], [6] without using
% cite.sty will become [1], [2], [5]--[7], [9] using cite.sty. cite.sty's
% \cite will automatically add leading space, if needed. Use cite.sty's
% noadjust option (cite.sty V3.8 and later) if you want to turn this off
% such as if a citation ever needs to be enclosed in parenthesis.
% cite.sty is already installed on most LaTeX systems. Be sure and use
% version 5.0 (2009-03-20) and later if using hyperref.sty.
% The latest version can be obtained at:
% http:__www.ctan.org_pkg_cite
% The documentation is contained in the cite.sty file itself.
%
% Note that some packages require special options to format as the Computer
% Society requires. In particular, Computer Society  papers do not use
% compressed citation ranges as is done in typical IEEE papers
% (e.g., [1]-[4]). Instead, they list every citation separately in order
% (e.g., [1], [2], [3], [4]). To get the latter we need to load the cite
% package with the nocompress option which is supported by cite.sty v4.0
% and later. Note also the use of a CLASSOPTION conditional provided by
% IEEEtran.cls V1.7 and later.

% *** GRAPHICS RELATED PACKAGES ***
%
\ifCLASSINFOpdf
  % \usepackage[pdftex]{graphicx}
  % declare the path(s) where your graphic files are
  % \graphicspath{{.._pdf_}{.._jpeg_}}
  % and their extensions so you won't have to specify these with
  % every instance of \includegraphics
  % \DeclareGraphicsExtensions{.pdf,.jpeg,.png}
\else
  % or other class option (dvipsone, dvipdf, if not using dvips). graphicx
  % will default to the driver specified in the system graphics.cfg if no
  % driver is specified.
  % \usepackage[dvips]{graphicx}
  % declare the path(s) where your graphic files are
  % \graphicspath{{.._eps_}}
  % and their extensions so you won't have to specify these with
  % every instance of \includegraphics
  % \DeclareGraphicsExtensions{.eps}
\fi
\hyphenation{op-tical net-works semi-conduc-tor}

\begin{document}
%
% paper title
% Titles are generally capitalized except for words such as a, an, and, as,
% at, but, by, for, in, nor, of, on, or, the, to and up, which are usually
% not capitalized unless they are the first or last word of the title.
% Linebreaks \\ can be used within to get better formatting as desired.
% Do not put math or special symbols in the title.
\title{Supplementary Material: \\
% Additional qualitative comparison of synthesized images with existing methods}
Geometry-Guided Street-View Panorama Synthesis from Satellite Imagery}
%
%
% author names and IEEE memberships
% note positions of commas and nonbreaking spaces ( ~ ) LaTeX will not break
% a structure at a ~ so this keeps an author's name from being broken across
% two lines.
% use \thanks{} to gain access to the first footnote area
% a separate \thanks must be used for each paragraph as LaTeX2e's \thanks
% was not built to handle multiple paragraphs
%
%
%\IEEEcompsocitemizethanks is a special \thanks that produces the bulleted
% lists the Computer Society journals use for "first footnote" author
% affiliations. Use \IEEEcompsocthanksitem which works much like \item
% for each affiliation group. When not in compsoc mode,
% \IEEEcompsocitemizethanks becomes like \thanks and
% \IEEEcompsocthanksitem becomes a line break with idention. This
% facilitates dual compilation, although admittedly the differences in the
% desired content of \author between the different types of papers makes a
% one-size-fits-all approach a daunting prospect. For instance, compsoc 
% journal papers have the author affiliations above the "Manuscript
% received ..."  text while in non-compsoc journals this is reversed. Sigh.

\author{Yujiao~Shi,
        Dylan~Campbell,
        Xin~Yu,
        and~Hongdong~Li
% \author{Michael~Shell,~\IEEEmembership{Member,~IEEE,}
%         John~Doe,~\IEEEmembership{Fellow,~OSA,}
%         and~Jane~Doe,~\IEEEmembership{Life~Fellow,~IEEE}% <-this % stops a space
% \IEEEcompsocitemizethanks{\IEEEcompsocthanksitem 
% Y. Shi, D. Campbell and H. Li are with the Australian National University, Canberra, ACT 2600, Australia, and also with the Australian Centre for Robotic Vision, Acton, ACT 2601, Australia. \protect\\%
% E-mail: \{yujiao.shi, dylan.campbell, hongdong.li\}@anu.edu.au.
% % note need leading \protect in front of \\ to get a newline within \thanks as
% % \\ is fragile and will error, could use \hfil\break instead.
% \IEEEcompsocthanksitem X. Yu is with the University of Technology Sydney.\protect\\
% E-mail: xin.yu@uts.edu.au}% <-this % stops an unwanted space
% % % \thanks{Manuscript received April 19, 2005; revised August 26, 2015.}
}

% The paper headers
\markboth{ }%
{ }

% \markboth{Journal of \LaTeX\ Class Files,~Vol.~14, No.~8, August~2015}%
% {Shell \MakeLowercase{\textit{et al.}}: Bare Demo of IEEEtran.cls for Computer Society Journals}

% make the title area
\maketitle

\begin{figure*}
    \setlength{\abovecaptionskip}{0pt}
    \setlength{\belowcaptionskip}{0pt}
    \centering
    % \subfloat[CVUSA]{
    \centering
    \begin{minipage}{0.1\linewidth}
    \parbox[][1.9cm][c]{\linewidth}{
    \includegraphics[width=\linewidth]{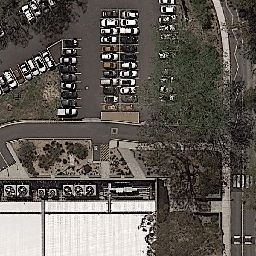}
    }
    \parbox[][1.9cm][c]{\linewidth}{
    \includegraphics[width=\linewidth]{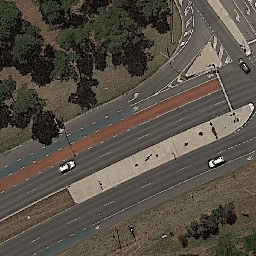}
    }
    \parbox[][1.9cm][c]{\linewidth}{
    \includegraphics[width=\linewidth]{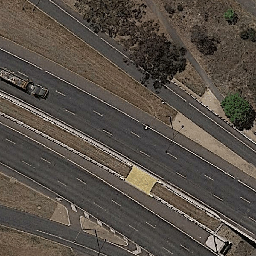}
    }
    \parbox[][1.9cm][c]{\linewidth}{
    \includegraphics[width=\linewidth]{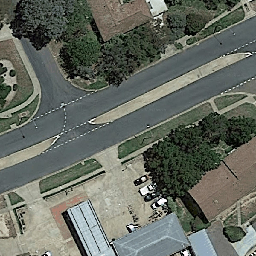}
    }
    \parbox[][1.9cm][c]{\linewidth}{
    \includegraphics[width=\linewidth]{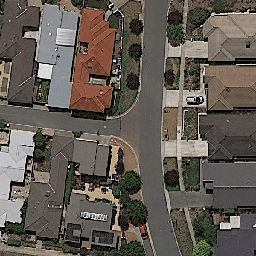}
    }
    \parbox[][1.9cm][c]{\linewidth}{
    \includegraphics[width=\linewidth]{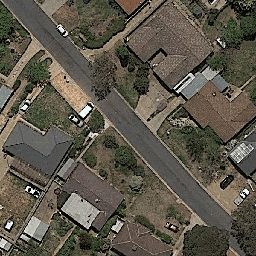}
    }
    \parbox[][1.9cm][c]{\linewidth}{
    \includegraphics[width=\linewidth]{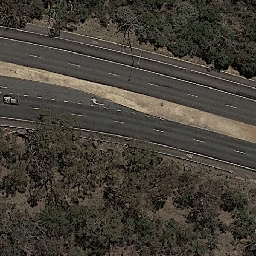}
    }
    \parbox[][1.9cm][c]{\linewidth}{
    \includegraphics[width=\linewidth]{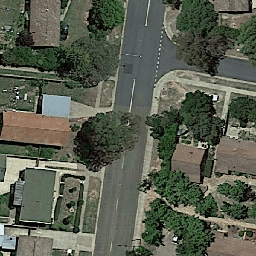}
    }
    \parbox[][1.9cm][c]{\linewidth}{
    \includegraphics[width=\linewidth]{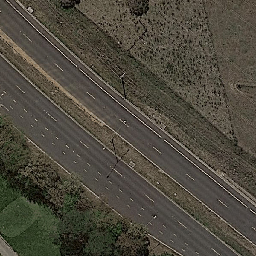}
    }
    \parbox[][1.9cm][c]{\linewidth}{
    \includegraphics[width=\linewidth]{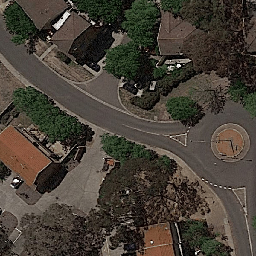}
    }
    \parbox[][1.9cm][c]{\linewidth}{
    \includegraphics[width=\linewidth]{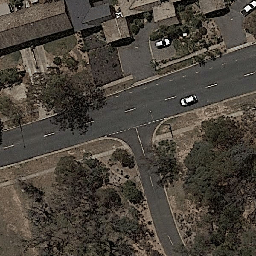}
    }
    \parbox[][1.9cm][c]{\linewidth}{
    \includegraphics[width=\linewidth]{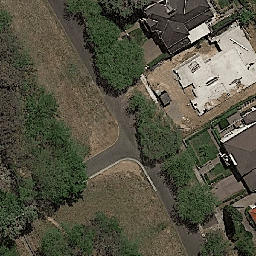}
    }
    \parbox[][1.9cm][c]{\linewidth}{
    \includegraphics[width=\linewidth]{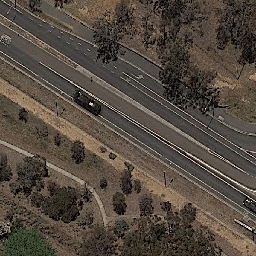}
    }\\
    \centerline{Satellite Image}
    \end{minipage}
    \centering
    \begin{minipage}{0.2\linewidth}
    \parbox[][1.9cm][c]{\linewidth}{
    \includegraphics[width=\linewidth, height=0.5\linewidth]{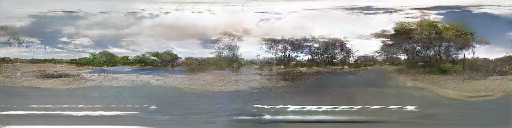}
    }
    \parbox[][1.9cm][c]{\linewidth}{
    \includegraphics[width=\linewidth, height=0.5\linewidth]{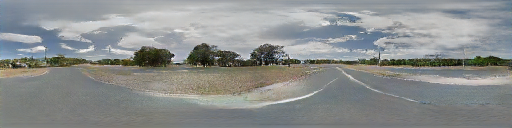}
    }
    \parbox[][1.9cm][c]{\linewidth}{
    \includegraphics[width=\linewidth, height=0.5\linewidth]{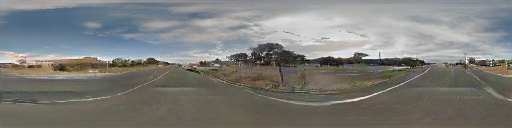}
    }
    \parbox[][1.9cm][c]{\linewidth}{
    \includegraphics[width=\linewidth, height=0.5\linewidth]{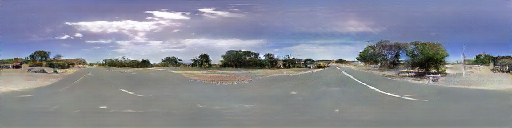}
    }
    \parbox[][1.9cm][c]{\linewidth}{
    \includegraphics[width=\linewidth, height=0.5\linewidth]{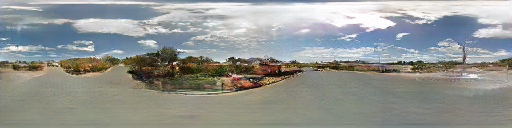}
    }
    \parbox[][1.9cm][c]{\linewidth}{
    \includegraphics[width=\linewidth, height=0.5\linewidth]{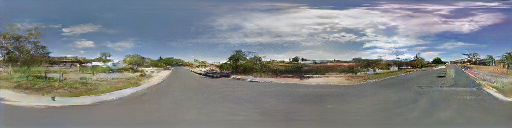}
    }
    \parbox[][1.9cm][c]{\linewidth}{
    \includegraphics[width=\linewidth, height=0.5\linewidth]{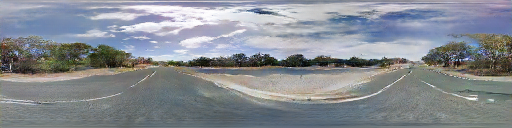}
    }
    \parbox[][1.9cm][c]{\linewidth}{
    \includegraphics[width=\linewidth, height=0.5\linewidth]{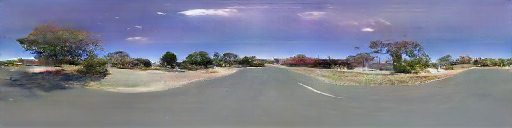}
    }
    \parbox[][1.9cm][c]{\linewidth}{
    \includegraphics[width=\linewidth, height=0.5\linewidth]{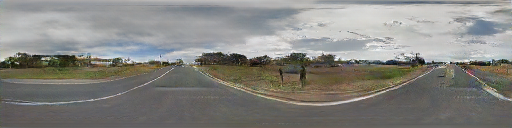}
    }
    \parbox[][1.9cm][c]{\linewidth}{
    \includegraphics[width=\linewidth, height=0.5\linewidth]{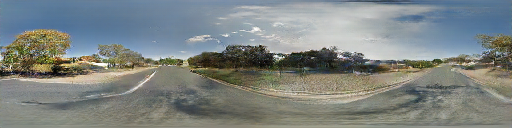}
    }
    \parbox[][1.9cm][c]{\linewidth}{
    \includegraphics[width=\linewidth, height=0.5\linewidth]{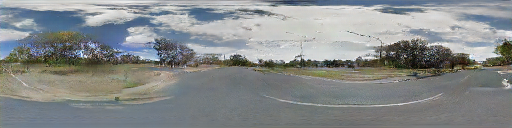}
    }
    \parbox[][1.9cm][c]{\linewidth}{
    \includegraphics[width=\linewidth, height=0.5\linewidth]{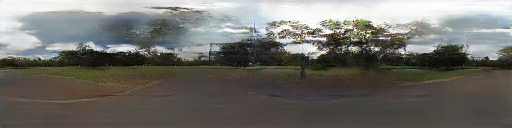}
    }
    \parbox[][1.9cm][c]{\linewidth}{
    \includegraphics[width=\linewidth, height=0.5\linewidth]{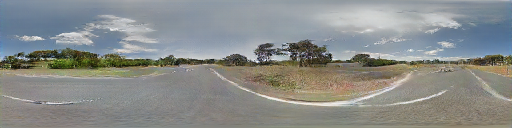}
    }\\
    \centerline{Pix2Pix}
    \end{minipage}
    \centering
    \begin{minipage}{0.2\linewidth}
    \parbox[][1.9cm][c]{\linewidth}{
    \includegraphics[width=\linewidth, height=0.5\linewidth]{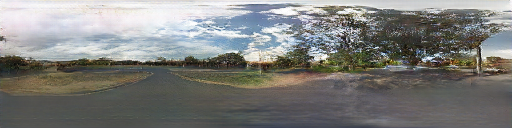}
    }
    \parbox[][1.9cm][c]{\linewidth}{
    \includegraphics[width=\linewidth, height=0.5\linewidth]{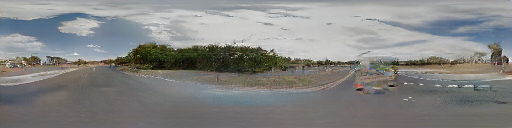}
    }
    \parbox[][1.9cm][c]{\linewidth}{
    \includegraphics[width=\linewidth, height=0.5\linewidth]{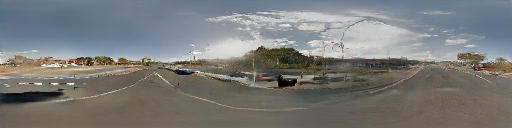}
    }
    \parbox[][1.9cm][c]{\linewidth}{
    \includegraphics[width=\linewidth, height=0.5\linewidth]{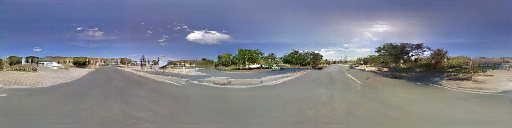}
    }
    \parbox[][1.9cm][c]{\linewidth}{
    \includegraphics[width=\linewidth, height=0.5\linewidth]{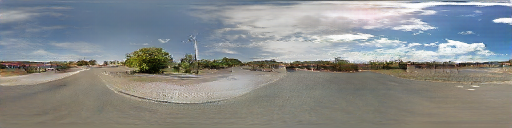}
    }
    \parbox[][1.9cm][c]{\linewidth}{
    \includegraphics[width=\linewidth, height=0.5\linewidth]{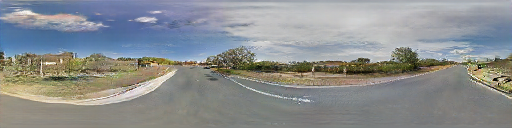}
    }
    \parbox[][1.9cm][c]{\linewidth}{
    \includegraphics[width=\linewidth, height=0.5\linewidth]{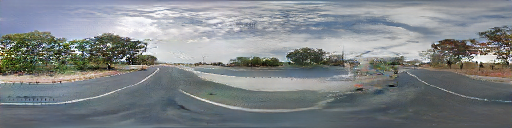}
    }
    \parbox[][1.9cm][c]{\linewidth}{
    \includegraphics[width=\linewidth, height=0.5\linewidth]{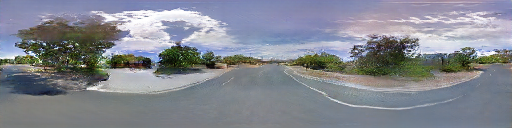}
    }
    \parbox[][1.9cm][c]{\linewidth}{
    \includegraphics[width=\linewidth, height=0.5\linewidth]{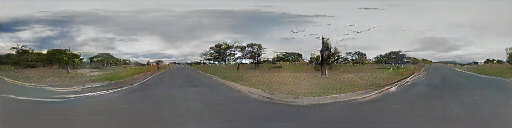}
    }
    \parbox[][1.9cm][c]{\linewidth}{
    \includegraphics[width=\linewidth, height=0.5\linewidth]{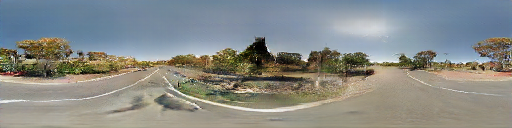}
    }
    \parbox[][1.9cm][c]{\linewidth}{
    \includegraphics[width=\linewidth, height=0.5\linewidth]{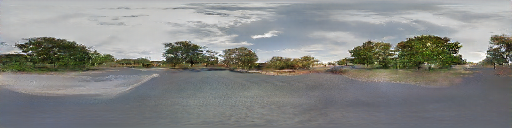}
    }
    \parbox[][1.9cm][c]{\linewidth}{
    \includegraphics[width=\linewidth, height=0.5\linewidth]{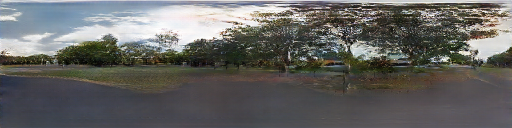}
    }
    \parbox[][1.9cm][c]{\linewidth}{
    \includegraphics[width=\linewidth, height=0.5\linewidth]{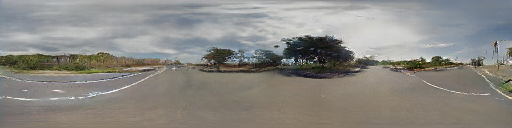}
    }\\
    \centerline{XFork}
    \end{minipage}
    % \label{projected aerial (additional)}
    \centering
    \begin{minipage}{0.2\linewidth}
    \parbox[][1.9cm][c]{\linewidth}{
    \includegraphics[width=\linewidth, height=0.5\linewidth]{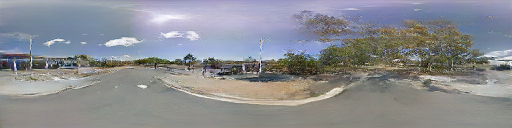}
    }
    \parbox[][1.9cm][c]{\linewidth}{
    \includegraphics[width=\linewidth, height=0.5\linewidth]{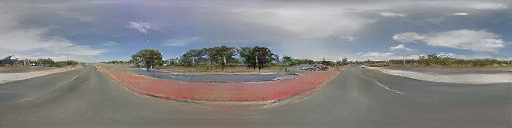}
    }
    \parbox[][1.9cm][c]{\linewidth}{
    \includegraphics[width=\linewidth, height=0.5\linewidth]{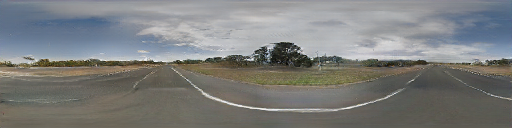}
    }
    \parbox[][1.9cm][c]{\linewidth}{
    \includegraphics[width=\linewidth, height=0.5\linewidth]{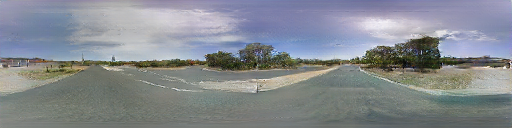}
    }
    \parbox[][1.9cm][c]{\linewidth}{
    \includegraphics[width=\linewidth, height=0.5\linewidth]{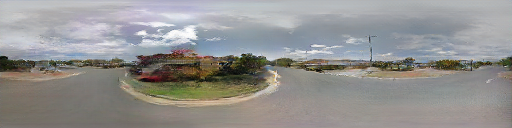}
    }
    \parbox[][1.9cm][c]{\linewidth}{
    \includegraphics[width=\linewidth, height=0.5\linewidth]{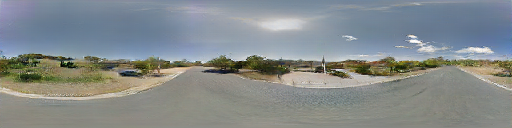}
    }
    \parbox[][1.9cm][c]{\linewidth}{
    \includegraphics[width=\linewidth, height=0.5\linewidth]{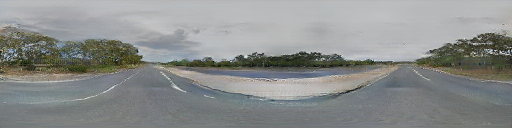}
    }
    \parbox[][1.9cm][c]{\linewidth}{
    \includegraphics[width=\linewidth, height=0.5\linewidth]{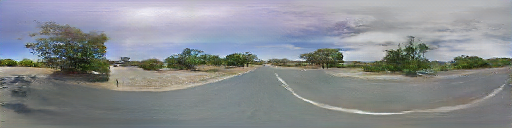}
    }
    \parbox[][1.9cm][c]{\linewidth}{
    \includegraphics[width=\linewidth, height=0.5\linewidth]{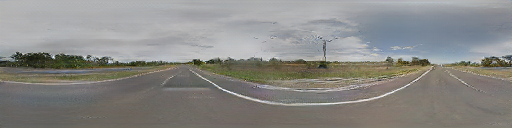}
    }
    \parbox[][1.9cm][c]{\linewidth}{
    \includegraphics[width=\linewidth, height=0.5\linewidth]{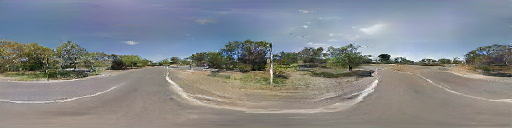}
    }
    \parbox[][1.9cm][c]{\linewidth}{
    \includegraphics[width=\linewidth, height=0.5\linewidth]{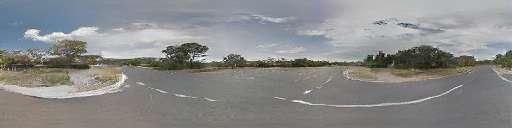}
    }
    \parbox[][1.9cm][c]{\linewidth}{
    \includegraphics[width=\linewidth, height=0.5\linewidth]{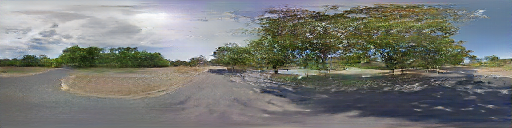}
    }
    \parbox[][1.9cm][c]{\linewidth}{
    \includegraphics[width=\linewidth, height=0.5\linewidth]{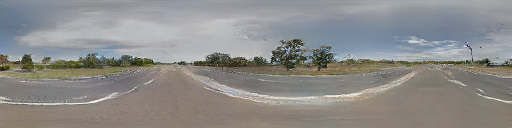}
    }\\
    \centerline{Ours}
    \end{minipage}
    \centering
    \begin{minipage}{0.2\linewidth}
    % \parbox[][1.9cm][c]{\linewidth}{
    % \includegraphics[width=\linewidth, height=0.5\linewidth]{images_results_CVACT_grd_0007081.png}
    % }
    \parbox[][1.9cm][c]{\linewidth}{
    \includegraphics[width=\linewidth, height=0.5\linewidth]{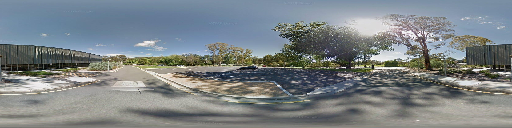}
    }
    \parbox[][1.9cm][c]{\linewidth}{
    \includegraphics[width=\linewidth, height=0.5\linewidth]{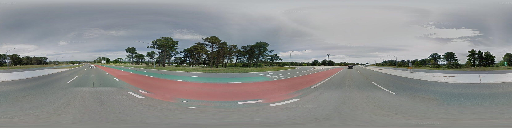}
    }
    \parbox[][1.9cm][c]{\linewidth}{
    \includegraphics[width=\linewidth, height=0.5\linewidth]{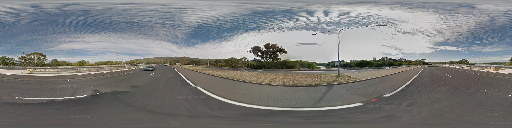}
    }
    \parbox[][1.9cm][c]{\linewidth}{
    \includegraphics[width=\linewidth, height=0.5\linewidth]{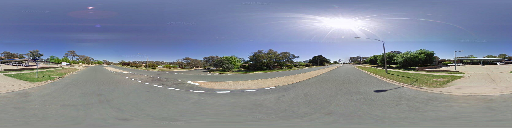}
    }
    \parbox[][1.9cm][c]{\linewidth}{
    \includegraphics[width=\linewidth, height=0.5\linewidth]{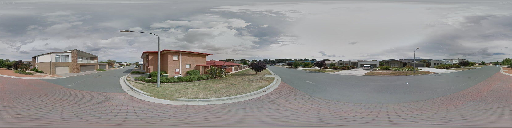}
    }
    \parbox[][1.9cm][c]{\linewidth}{
    \includegraphics[width=\linewidth, height=0.5\linewidth]{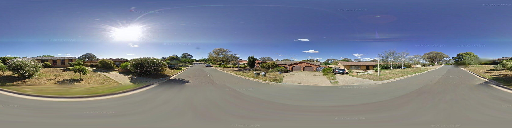}
    }
    \parbox[][1.9cm][c]{\linewidth}{
    \includegraphics[width=\linewidth, height=0.5\linewidth]{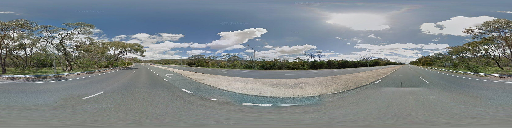}
    }
    \parbox[][1.9cm][c]{\linewidth}{
    \includegraphics[width=\linewidth, height=0.5\linewidth]{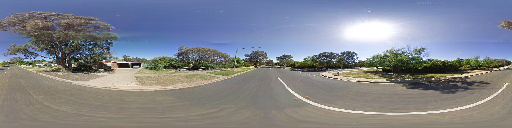}
    }
    \parbox[][1.9cm][c]{\linewidth}{
    \includegraphics[width=\linewidth, height=0.5\linewidth]{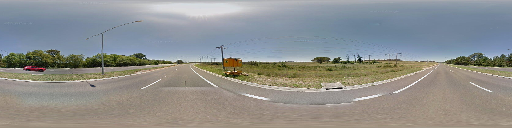}
    }
    \parbox[][1.9cm][c]{\linewidth}{
    \includegraphics[width=\linewidth, height=0.5\linewidth]{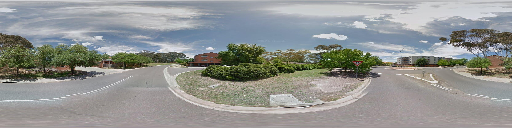}
    }
    \parbox[][1.9cm][c]{\linewidth}{
    \includegraphics[width=\linewidth, height=0.5\linewidth]{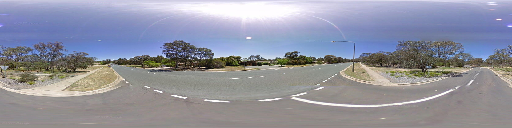}
    }
    \parbox[][1.9cm][c]{\linewidth}{
    \includegraphics[width=\linewidth, height=0.5\linewidth]{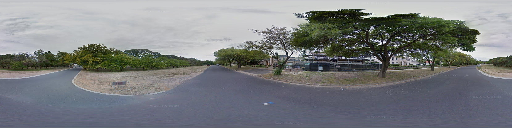}
    }
    \parbox[][1.9cm][c]{\linewidth}{
    \includegraphics[width=\linewidth, height=0.5\linewidth]{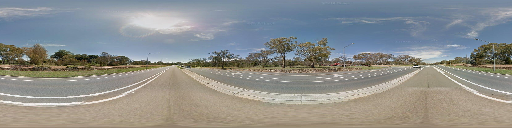}
    }\\
    \centerline{Ground Truth}
    \end{minipage}
    % }
    \caption{ Additional qualitative comparison of synthesized images on the CVACT dataset.
    }
    \label{fig:Qualitative CVACT}
\end{figure*}

\begin{figure*}
    \setlength{\abovecaptionskip}{0pt}
    \setlength{\belowcaptionskip}{0pt}
    \centering
    % \subfloat[CVUSA]{
    \centering
    \begin{minipage}{0.1\linewidth}
    \parbox[][1.9cm][c]{\linewidth}{
    \includegraphics[width=\linewidth]{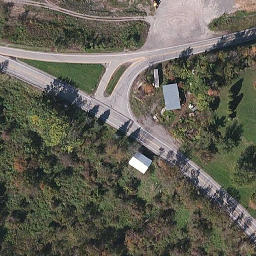}
    }
    \parbox[][1.9cm][c]{\linewidth}{
    \includegraphics[width=\linewidth]{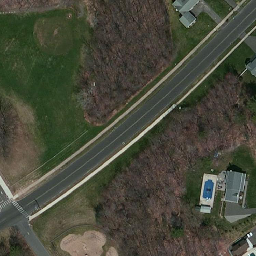}
    }
    \parbox[][1.9cm][c]{\linewidth}{
    \includegraphics[width=\linewidth]{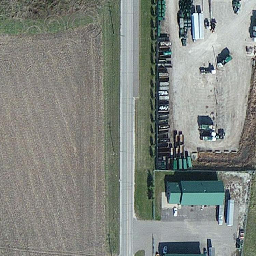}
    }
    \parbox[][1.9cm][c]{\linewidth}{
    \includegraphics[width=\linewidth]{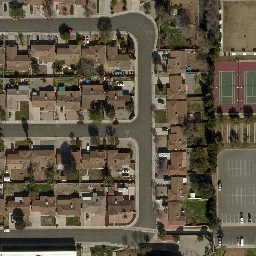}
    }
    \parbox[][1.9cm][c]{\linewidth}{
    \includegraphics[width=\linewidth]{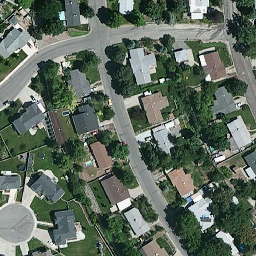}
    }
    \parbox[][1.9cm][c]{\linewidth}{
    \includegraphics[width=\linewidth]{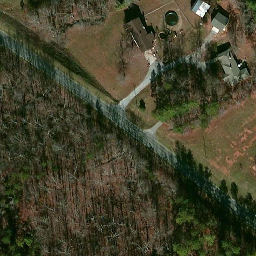}
    }
    \parbox[][1.9cm][c]{\linewidth}{
    \includegraphics[width=\linewidth]{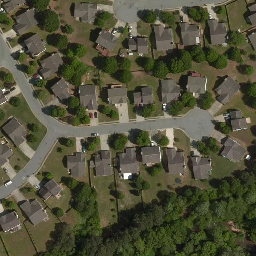}
    }
    \parbox[][1.9cm][c]{\linewidth}{
    \includegraphics[width=\linewidth]{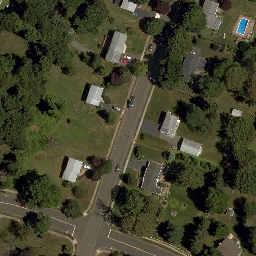}
    }
    \parbox[][1.9cm][c]{\linewidth}{
    \includegraphics[width=\linewidth]{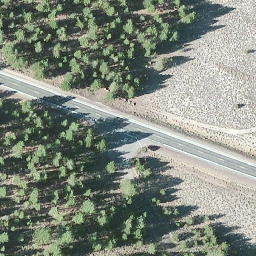}
    }
    \parbox[][1.9cm][c]{\linewidth}{
    \includegraphics[width=\linewidth]{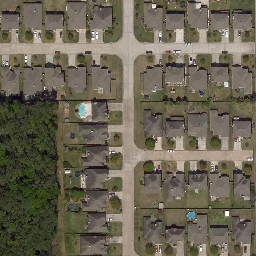}
    }
    \parbox[][1.9cm][c]{\linewidth}{
    \includegraphics[width=\linewidth]{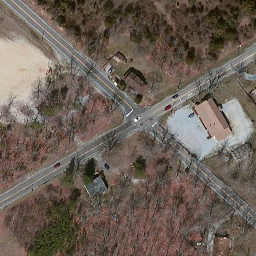}
    }
    \parbox[][1.9cm][c]{\linewidth}{
    \includegraphics[width=\linewidth]{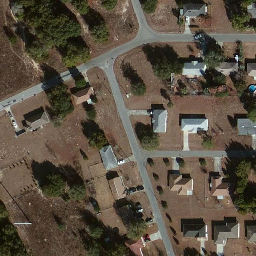}
    }
    \parbox[][1.9cm][c]{\linewidth}{
    \includegraphics[width=\linewidth]{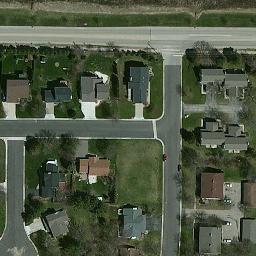}
    }\\
    \centerline{Satellite Image}
    \end{minipage}
    \centering
    \begin{minipage}{0.2\linewidth}
    \parbox[][1.9cm][c]{\linewidth}{
    \includegraphics[width=\linewidth, height=0.5\linewidth]{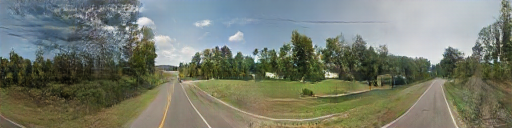}
    }
    \parbox[][1.9cm][c]{\linewidth}{
    \includegraphics[width=\linewidth, height=0.5\linewidth]{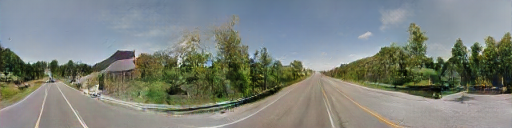}
    }
    \parbox[][1.9cm][c]{\linewidth}{
    \includegraphics[width=\linewidth, height=0.5\linewidth]{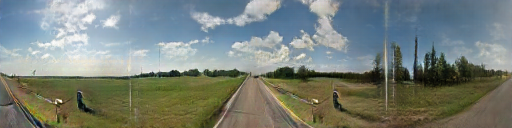}
    }
    \parbox[][1.9cm][c]{\linewidth}{
    \includegraphics[width=\linewidth, height=0.5\linewidth]{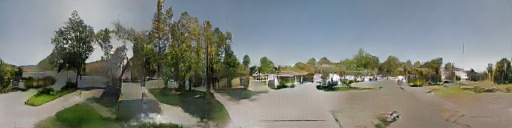}
    }
    \parbox[][1.9cm][c]{\linewidth}{
    \includegraphics[width=\linewidth, height=0.5\linewidth]{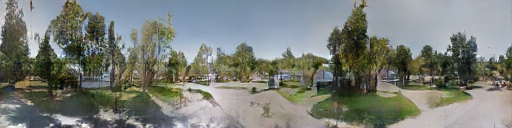}
    }
    \parbox[][1.9cm][c]{\linewidth}{
    \includegraphics[width=\linewidth, height=0.5\linewidth]{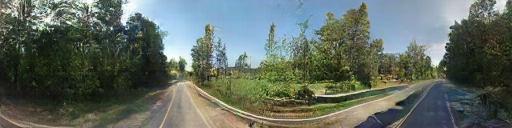}
    }
    \parbox[][1.9cm][c]{\linewidth}{
    \includegraphics[width=\linewidth, height=0.5\linewidth]{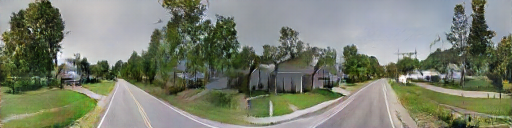}
    }
    \parbox[][1.9cm][c]{\linewidth}{
    \includegraphics[width=\linewidth, height=0.5\linewidth]{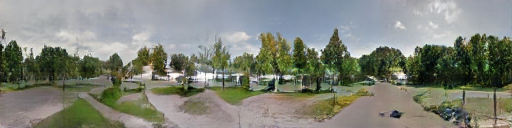}
    }
    \parbox[][1.9cm][c]{\linewidth}{
    \includegraphics[width=\linewidth, height=0.5\linewidth]{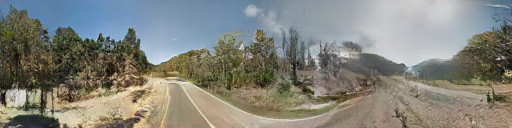}
    }
    \parbox[][1.9cm][c]{\linewidth}{
    \includegraphics[width=\linewidth, height=0.5\linewidth]{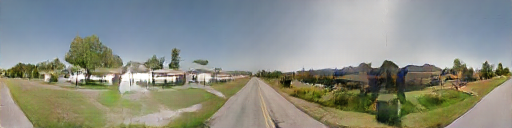}
    }
    \parbox[][1.9cm][c]{\linewidth}{
    \includegraphics[width=\linewidth, height=0.5\linewidth]{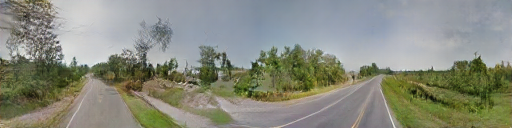}
    }
    \parbox[][1.9cm][c]{\linewidth}{
    \includegraphics[width=\linewidth, height=0.5\linewidth]{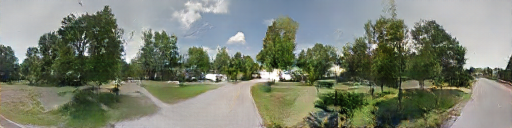}
    }
    \parbox[][1.9cm][c]{\linewidth}{
    \includegraphics[width=\linewidth, height=0.5\linewidth]{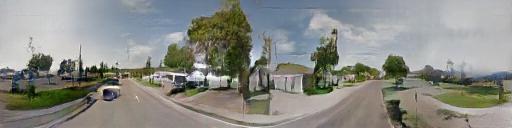}
    }\\
    \centerline{Pix2Pix}
    \end{minipage}
    \centering
    \begin{minipage}{0.2\linewidth}
    \parbox[][1.9cm][c]{\linewidth}{
    \includegraphics[width=\linewidth, height=0.5\linewidth]{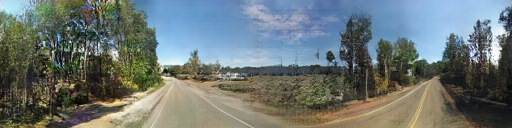}
    }
    \parbox[][1.9cm][c]{\linewidth}{
    \includegraphics[width=\linewidth, height=0.5\linewidth]{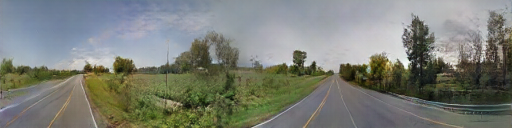}
    }
    \parbox[][1.9cm][c]{\linewidth}{
    \includegraphics[width=\linewidth, height=0.5\linewidth]{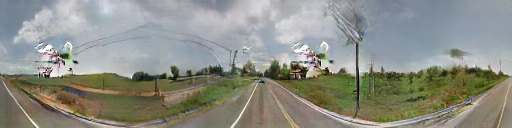}
    }
    \parbox[][1.9cm][c]{\linewidth}{
    \includegraphics[width=\linewidth, height=0.5\linewidth]{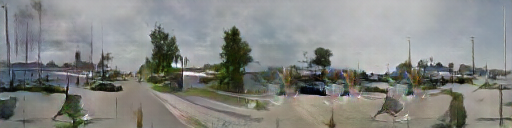}
    }
    \parbox[][1.9cm][c]{\linewidth}{
    \includegraphics[width=\linewidth, height=0.5\linewidth]{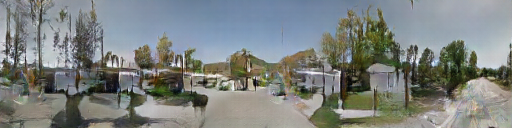}
    }
    \parbox[][1.9cm][c]{\linewidth}{
    \includegraphics[width=\linewidth, height=0.5\linewidth]{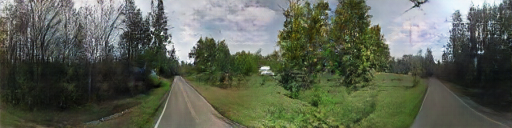}
    }
    \parbox[][1.9cm][c]{\linewidth}{
    \includegraphics[width=\linewidth, height=0.5\linewidth]{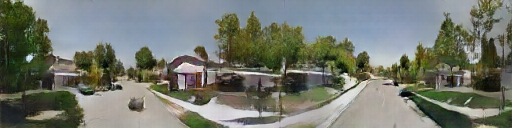}
    }
    \parbox[][1.9cm][c]{\linewidth}{
    \includegraphics[width=\linewidth, height=0.5\linewidth]{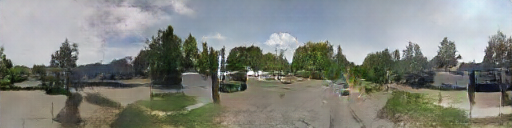}
    }
    \parbox[][1.9cm][c]{\linewidth}{
    \includegraphics[width=\linewidth, height=0.5\linewidth]{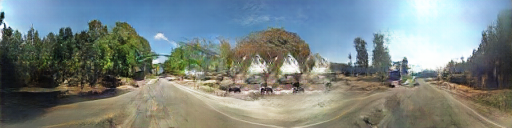}
    }
    \parbox[][1.9cm][c]{\linewidth}{
    \includegraphics[width=\linewidth, height=0.5\linewidth]{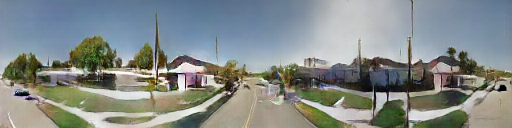}
    }
    \parbox[][1.9cm][c]{\linewidth}{
    \includegraphics[width=\linewidth, height=0.5\linewidth]{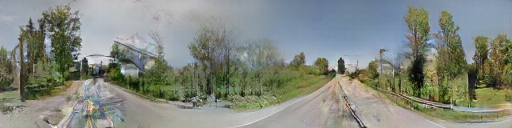}
    }
    \parbox[][1.9cm][c]{\linewidth}{
    \includegraphics[width=\linewidth, height=0.5\linewidth]{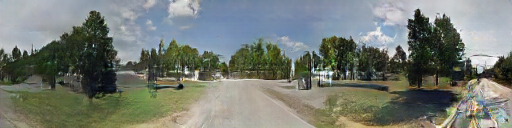}
    }
    \parbox[][1.9cm][c]{\linewidth}{
    \includegraphics[width=\linewidth, height=0.5\linewidth]{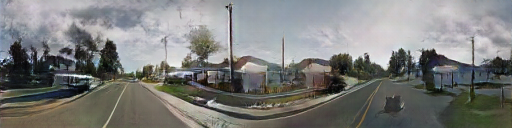}
    }\\
    \centerline{XFork}
    \end{minipage}
    % \label{projected aerial (additional)}
    \centering
    \begin{minipage}{0.2\linewidth}
    % \parbox[][1.9cm][c]{\linewidth}{
    % \includegraphics[width=\linewidth, height=0.5\linewidth]{images_results_CVUSA_ourslper_0007081.png}
    % }
    \parbox[][1.9cm][c]{\linewidth}{
    \includegraphics[width=\linewidth, height=0.5\linewidth]{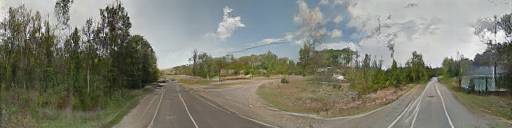}
    }
    \parbox[][1.9cm][c]{\linewidth}{
    \includegraphics[width=\linewidth, height=0.5\linewidth]{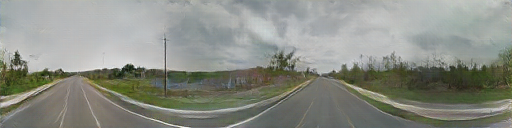}
    }
    \parbox[][1.9cm][c]{\linewidth}{
    \includegraphics[width=\linewidth, height=0.5\linewidth]{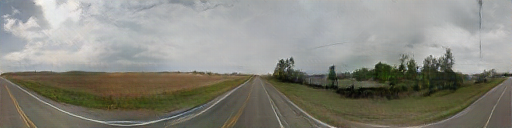}
    }
    \parbox[][1.9cm][c]{\linewidth}{
    \includegraphics[width=\linewidth, height=0.5\linewidth]{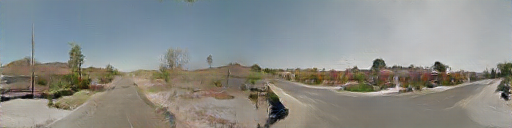}
    }
    \parbox[][1.9cm][c]{\linewidth}{
    \includegraphics[width=\linewidth, height=0.5\linewidth]{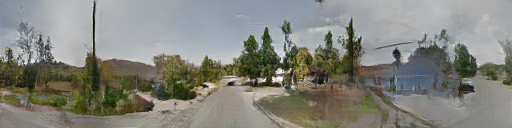}
    }
    \parbox[][1.9cm][c]{\linewidth}{
    \includegraphics[width=\linewidth, height=0.5\linewidth]{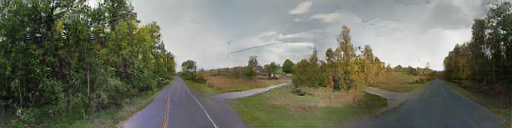}
    }
    \parbox[][1.9cm][c]{\linewidth}{
    \includegraphics[width=\linewidth, height=0.5\linewidth]{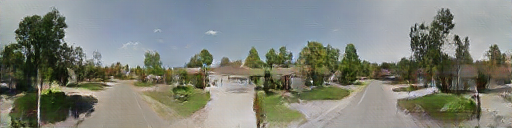}
    }
    \parbox[][1.9cm][c]{\linewidth}{
    \includegraphics[width=\linewidth, height=0.5\linewidth]{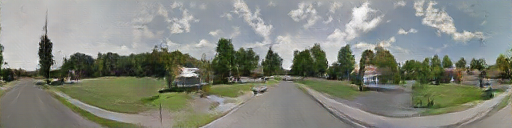}
    }
    \parbox[][1.9cm][c]{\linewidth}{
    \includegraphics[width=\linewidth, height=0.5\linewidth]{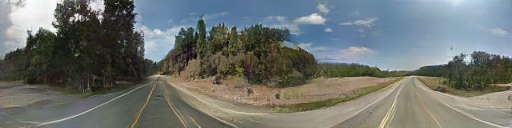}
    }
    \parbox[][1.9cm][c]{\linewidth}{
    \includegraphics[width=\linewidth, height=0.5\linewidth]{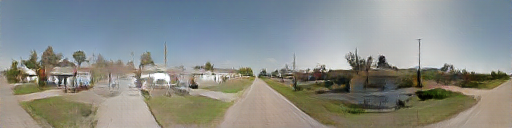}
    }
    \parbox[][1.9cm][c]{\linewidth}{
    \includegraphics[width=\linewidth, height=0.5\linewidth]{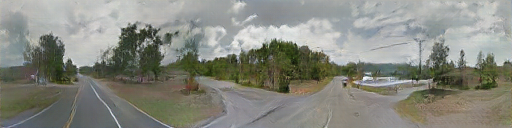}
    }
    \parbox[][1.9cm][c]{\linewidth}{
    \includegraphics[width=\linewidth, height=0.5\linewidth]{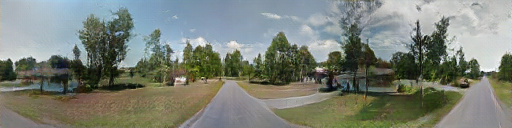}
    }
    \parbox[][1.9cm][c]{\linewidth}{
    \includegraphics[width=\linewidth, height=0.5\linewidth]{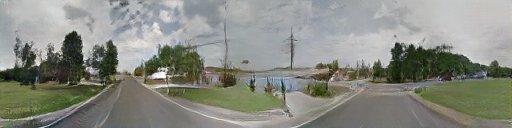}
    }\\
    \centerline{Ours}
    \end{minipage}
    \centering
    \begin{minipage}{0.2\linewidth}
    \parbox[][1.9cm][c]{\linewidth}{
    \includegraphics[width=\linewidth, height=0.5\linewidth]{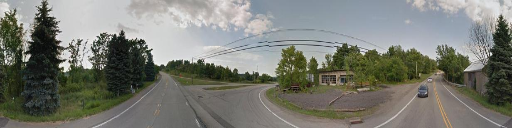}
    }
    \parbox[][1.9cm][c]{\linewidth}{
    \includegraphics[width=\linewidth, height=0.5\linewidth]{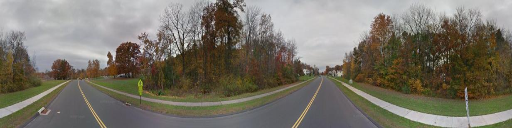}
    }
    \parbox[][1.9cm][c]{\linewidth}{
    \includegraphics[width=\linewidth, height=0.5\linewidth]{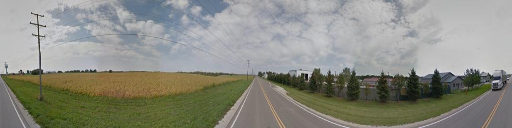}
    }
    \parbox[][1.9cm][c]{\linewidth}{
    \includegraphics[width=\linewidth, height=0.5\linewidth]{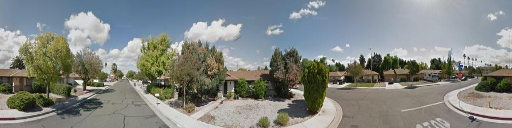}
    }
    \parbox[][1.9cm][c]{\linewidth}{
    \includegraphics[width=\linewidth, height=0.5\linewidth]{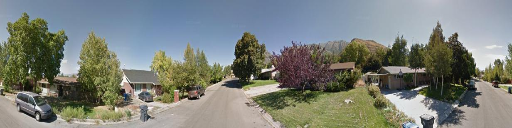}
    }
    \parbox[][1.9cm][c]{\linewidth}{
    \includegraphics[width=\linewidth, height=0.5\linewidth]{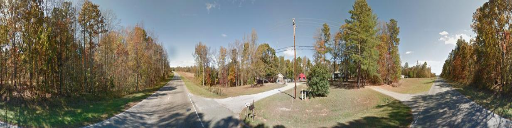}
    }
    \parbox[][1.9cm][c]{\linewidth}{
    \includegraphics[width=\linewidth, height=0.5\linewidth]{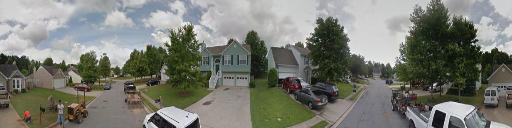}
    }
    \parbox[][1.9cm][c]{\linewidth}{
    \includegraphics[width=\linewidth, height=0.5\linewidth]{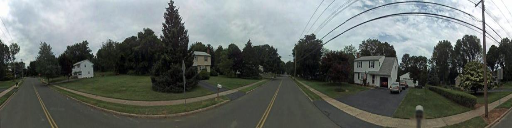}
    }
    \parbox[][1.9cm][c]{\linewidth}{
    \includegraphics[width=\linewidth, height=0.5\linewidth]{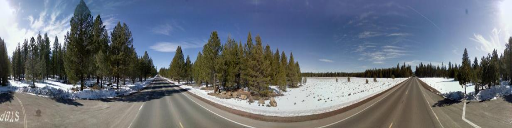}
    }
    \parbox[][1.9cm][c]{\linewidth}{
    \includegraphics[width=\linewidth, height=0.5\linewidth]{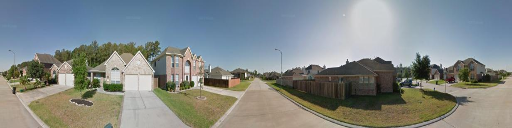}
    }
    \parbox[][1.9cm][c]{\linewidth}{
    \includegraphics[width=\linewidth, height=0.5\linewidth]{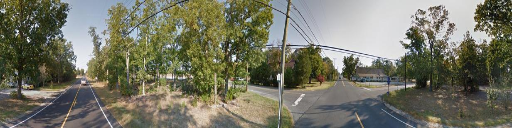}
    }
    \parbox[][1.9cm][c]{\linewidth}{
    \includegraphics[width=\linewidth, height=0.5\linewidth]{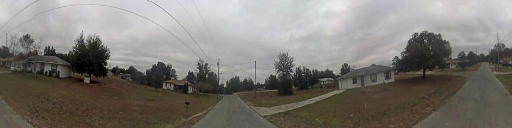}
    }
    \parbox[][1.9cm][c]{\linewidth}{
    \includegraphics[width=\linewidth, height=0.5\linewidth]{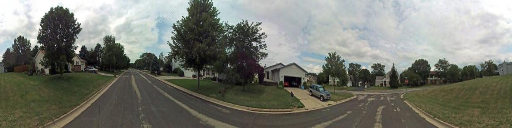}
    }\\
    \centerline{Ground Truth}
    \end{minipage}
    % }
    \caption{ Additional qualitative comparison of synthesized images on the CVUSA dataset.
    }
    \label{fig:Qualitative abla2}
\end{figure*}

\end{document}
